# Supplementary material for: An Investigation of Prompt Variations for Zero-shot LLM-based Rankers
Source: arXiv:2406.14117 source file (2025-07-25)
Supplement: Supplementary file 1 [file appendix.tex]

%\newpage
%\section{Original Prompts of LLM rankers}
%\label{app_original_prompts}
%
%\begin{table*}[t!]
%	%\begin{tabular}{|l|l|l|l|l|l|l|l|}
%	\scriptsize
%	\centering
%	\caption{The content of each original prompt is structured with specific placeholders enclosed in braces ``\{\}''. For instance, ``\{query\}'' represents the query text. }
%	\label{table_orig_prompts}
%	\resizebox{1\textwidth}{!}{  
%		\begin{tabular}{@{}l|llll@{}}
%			\toprule
%			Rankers &
%			\multicolumn{1}{l|}{Original Prompt 1} &
%			\multicolumn{1}{l|}{Original Prompt 2} &
%			\multicolumn{1}{l|}{Original Prompt 3} &
%			Original Prompt 4 \\ \midrule
%			Pointwise &
%			\multicolumn{1}{l|}{\begin{tabular}[c]{@{}l@{}}Query: \{query\}\\ Passage: \{text\}\\ Does the passage answer the query?\\ Answer 'Yes' or 'No'\end{tabular}} &
%			\multicolumn{1}{l|}{\begin{tabular}[c]{@{}l@{}}Passage: \{text\}\\ Query: \{query\}\\ Is this passage relevant to the query?\\ Please answer True/False. Answer:\end{tabular}} &
%			\multicolumn{1}{l|}{\begin{tabular}[c]{@{}l@{}}For the following query and document, \\ judge whether they are 'Highly Relevant', 'Somewhat Relevant', or 'Not Relevant'.\\ Query: \{query\}\\ Document:\{text\}\\ Output:\end{tabular}} &
%			\begin{tabular}[c]{@{}l@{}}From a scale of 0 to 4, \\ judge the relevance between the query and the document.\\ Query: \{query\} \\ Document:\{text\} \\ Output:\end{tabular} \\ \midrule
%			Pairwise &
%			\multicolumn{4}{l}{\begin{tabular}[c]{@{}l@{}}Given a query: \{query\}, which of the following two passages is more relevant to the query? \\ Passage A: \{doc1\} \\ Passage B: \{doc2\} \\ Output Passage A or Passage B:\end{tabular}} \\ \midrule
%			Listwise &
%			\multicolumn{1}{l|}{\begin{tabular}[c]{@{}l@{}}\{Several Passages\} \\ Query = \{query\}\\ Passages = {[}Passage 1, Passage2, Passage3, Passage4{]} \\ Sort the Passages by their relevance to the Query. \\ Sorted Passages = {[}\end{tabular}} &
%			\multicolumn{3}{l}{\begin{tabular}[c]{@{}l@{}}You are RankGPT, an intelligent assistant that can rank passages based on their relevancy to the query. \\ I will provide you with \{num\} passages, each indicated by number identifier {[}{]}. \\ Rank the passages based on their relevance to query: \{query\}\\ \{Several Passages\} \\ Search Query: \{query\}. \\ Rank the \{num\} passages above based on their relevance to the search query. \\ The passages should be listed in descending order using identifiers. \\ The most relevant passages should be listed first. The output format should be {[}{]} $>$ {[}{]}, e.g., {[}1{]} $>$ {[}2{]}. \\ Only response the ranking results, do not say any word or explain.\end{tabular}} \\ \midrule
%			Setwise &
%			\multicolumn{4}{l}{\begin{tabular}[c]{@{}l@{}}Given a query "\{query\}", which of the following passages is the most relevant one to the query?\\ Passages [Passage A, Passage B, Passage C]\\ Output only the passage label of the most relevant passage:\end{tabular}} \\ \bottomrule
%		\end{tabular}
%	}
%\end{table*}


%The original prompts associated to each LLM ranking method are reported in Table~\ref{table_orig_prompts}; these prompts were collected from the works of \cite{zhuang2023beyond,qin2023large,ma2023zero,sun2023chatgpt,tang2023found,zhuang2023setwise},.
%
%In the original prompts for listwise the number of passages included in a single prompt is a parameter of the method. All passages included are denoted by ``\{Several Passages\}'', and ``\{num\}'' indicates the actual number of passages. Furthermore, in the first original listwise prompt, there is an instruction specifying the format as follows: ``Passages = {[}Passage 1, Passage 2, Passage 3, Passage 4{]}''. It is important to note that these entries are placeholders, not actual passages, and their count is determined by ``\{num\}''.





%\section{Best Prompt Variations}
%\label{app_best_prompts}
%Table~\ref{tab:best-settings-of-adjusted-prompt} reports the template combinations that lead to the best performing prompts across combinations of ranking method, LLM backbones, and dataset.

%\begin{table*}[t]
%	\centering
%	\caption{Prompt templates containing the components that lead to the most effective results across combinations of ranking method, LLM backbones, and dataset.}
%	\label{tab:best-settings-of-adjusted-prompt}
%	
%	\begin{subtable}{\textwidth}
%		\centering
%		\caption{Dataset: DL19}
%		\resizebox{\textwidth}{!}{
%			\begin{tabular}{@{}lc|c|c|c@{}}
%				\toprule
%				Model & Pointwise & Pairwise & Listwise & Setwise \\ \midrule
%				FlanT5-large & \makecell{TI\_3, OT\_1, \\ TW\_0, PF, B, RP\_1} & \makecell{TI\_1, OT\_1, \\ TW\_4, QF, B, RP\_None} & \makecell{TI\_3, OT\_2, \\ TW\_2, PF, E, RP\_None} & \makecell{TI\_1, OT\_3, \\ TW\_0, QF, B, RP\_None} \\ \midrule
%				FlanT5-xl & \makecell{TI\_2, OT\_3, \\ TW\_4, PF, E, RP\_1} & \makecell{TI\_1, OT\_1, \\ TW\_2, QF, B, RP\_1} & \makecell{TI\_3, OT\_2, \\ TW\_3, QF, B, RP\_None} & \makecell{TI\_1, OT\_3, \\ TW\_3, QF, E, RP\_1} \\ \midrule
%				FlanT5-xxl & \makecell{TI\_4, OT\_3, \\ TW\_1, PF, B, RP\_None} & \makecell{TI\_1, OT\_1, \\ TW\_0, QF, E, RP\_1} & \makecell{TI\_1, OT\_2, \\ TW\_2, QF, B, RP\_None} & \makecell{TI\_1, OT\_1, \\ TW\_4, QF, B, RP\_1} \\ \midrule
%				Mistral-7B & \makecell{TI\_1, OT\_4, \\ TW\_3, PF, E, RP\_1} & \makecell{TI\_1, OT\_1, \\ TW\_0, QF, E, RP\_1} & \makecell{TI\_1, OT\_1, \\ TW\_2, QF, B, RP\_None} & \makecell{TI\_1, OT\_3, \\ TW\_0, QF, E, RP\_1} \\ \midrule
%				Llama3-8B & \makecell{TI\_2, OT\_3, \\ TW\_2, PF, B, RP\_1} & \makecell{TI\_1, OT\_1, \\ TW\_0, QF, B, RP\_None} & \makecell{TI\_1, OT\_2, \\ TW\_0, QF, B, RP\_None} & \makecell{TI\_1, OT\_1, \\ TW\_3, PF, E, RP\_None} \\ 
%				\bottomrule
%			\end{tabular}
%		}
%	\end{subtable}
%	
%	\vspace{1em} % Add some vertical space between the subtables
%	
%	\begin{subtable}{\textwidth}
%		\centering
%		\caption{Dataset: DL20}
%		\resizebox{\textwidth}{!}{
%			\begin{tabular}{@{}lcccc@{}}
%				\toprule
%				Model & Pointwise & Pairwise & Listwise & Setwise \\ \midrule
%				FlanT5-large & \makecell{TI\_3, OT\_3, \\ TW\_3, PF, B, RP\_1} & \makecell{TI\_1, OT\_1, \\ TW\_2, PF, E, RP\_None} & \makecell{TI\_3, OT\_2, \\ TW\_1, PF, E, RP\_None} & \makecell{TI\_1, OT\_1, \\ TW\_2, PF, E, RP\_1} \\ \midrule
%				FlanT5-xl & \makecell{TI\_3, OT\_3, \\ TW\_4, QF, B, RP\_1} & \makecell{TI\_1, OT\_1, \\ TW\_5, QF, B, RP\_1} & \makecell{TI\_2, OT\_2, \\ TW\_3, PF, E, RP\_1} & \makecell{TI\_1, OT\_2, \\ TW\_5, PF, B, RP\_None} \\ \midrule
%				FlanT5-xxl & \makecell{TI\_3, OT\_1, \\ TW\_3, PF, B, RP\_None} & \makecell{TI\_1, OT\_1, \\ TW\_2, PF, E, RP\_1} & \makecell{TI\_2, OT\_2, \\ TW\_3, PF, B, RP\_None} & \makecell{TI\_1, OT\_3, \\ TW\_3, PF, B, RP\_1} \\ \midrule
%				Mistral-7B & \makecell{TI\_1, OT\_4, \\ TW\_2, PF, E, RP\_1} & \makecell{TI\_1, OT\_1, \\ TW\_1, QF, E, RP\_None} & \makecell{TI\_3, OT\_1, \\ TW\_0, QF, B, RP\_1} & \makecell{TI\_1, OT\_3, \\ TW\_2, QF, E, RP\_1} \\ \midrule
%				Llama3-8B & \makecell{TI\_1, OT\_3, \\ TW\_1, PF, B, RP\_1} & \makecell{TI\_1, OT\_1, \\ TW\_3, PF, E, RP\_1} & \makecell{TI\_3, OT\_2, \\ TW\_0, QF, B, RP\_None} & \makecell{TI\_1, OT\_2, \\ TW\_4, PF, E, RP\_None} \\
%				\bottomrule
%			\end{tabular}
%		}
%	\end{subtable}
%	
%	\vspace{1em} % Add some vertical space between the subtables
%	
%	\begin{subtable}{\textwidth}
%		\centering
%		\caption{Dataset: COVID}
%		\resizebox{\textwidth}{!}{
%			\begin{tabular}{@{}lcccc@{}}
%				\toprule
%				Model & Pointwise & Pairwise & Listwise & Setwise \\ \midrule
%				FlanT5-large & \makecell{TI\_3, OT\_1, \\ TW\_1, PF, B, RP\_1} & \makecell{TI\_1, OT\_1, \\ TW\_5, PF, B, RP\_1} & \makecell{TI\_3, OT\_2, \\ TW\_4, PF, E, RP\_None} & \makecell{TI\_1, OT\_1, \\ TW\_1, PF, B, RP\_None} \\ \midrule
%				FlanT5-xl & \makecell{TI\_3, OT\_1, \\ TW\_1, PF, B, RP\_1} & \makecell{TI\_1, OT\_1, \\ TW\_5, PF, B, RP\_1} & \makecell{TI\_2, OT\_2, \\ TW\_1, QF, E, RP\_None} & \makecell{TI\_1, OT\_3, \\ TW\_5, QF, E, RP\_None} \\ \midrule
%				FlanT5-xxl & \makecell{TI\_3, OT\_1, \\ TW\_1, PF, B, RP\_None} & \makecell{TI\_1, OT\_1, \\ TW\_0, PF, B, RP\_1} & \makecell{TI\_1, OT\_2, \\ TW\_3, PF, B, RP\_None} & \makecell{TI\_1, OT\_3, \\ TW\_5, PF, B, RP\_1} \\ \midrule
%				Mistral-7B & \makecell{TI\_2, OT\_2, \\ TW\_4, PF, B, RP\_1} & \makecell{TI\_1, OT\_1, \\ TW\_3, QF, B, RP\_1} & \makecell{TI\_1, OT\_1, \\ TW\_4, QF, B, RP\_None} & \makecell{TI\_1, OT\_1, \\ TW\_2, QF, B, RP\_None} \\ \midrule
%				Llama3-8B & \makecell{TI\_2, OT\_3, \\ TW\_5, QF, E, RP\_1} & \makecell{TI\_1, OT\_1, \\ TW\_4, QF, B, RP\_None} & \makecell{TI\_1, OT\_2, \\ TW\_0, QF, B, RP\_None} & \makecell{TI\_1, OT\_3, \\ TW\_1, QF, B, RP\_1} \\ 
%				\bottomrule
%			\end{tabular}
%		}
%	\end{subtable}
%	
%\end{table*}

%\modified{All words in appendix are just for insights. I have put them in my thesis, so you may use it as a start of idea.}
%\modified{
%We next consider the role of ranking algorithm instructions within various ranking families that offer multiple options for rank adjustments. Our analysis is structured around four principal aspects derived from the data presented in Table \ref{tab:best-settings-of-adjusted-prompt}: (1) Ranker-Specific Instruction, which includes Task Instruction (TI) and Output Type (OT); (2) Tone Words (TW); (3) Ordering, which encompasses Evidence Order (EO) and Position of Evidence (PE); and (4) Role Playing (RP). From these dimensions, several observations can be drawn (see below).}
%\subsection*{Ranker-Specific Instruction}
%Given the variability of Task Instruction (TI) and Output Type (OT) across different rankers, it is crucial to analyze these elements both jointly and separately within each ranking category.
%\begin{itemize}
%	\item \textbf{Pointwise Ranking:}
%	\begin{itemize}
%		\item TI\_3 emerges as the most effective task instruction, appearing as the best option in 7 out of 15 cases. This suggests a strong alignment between TI\_3 and the pointwise ranking objectives.
%		\item TI\_2 and TI\_1 also demonstrate moderate efficacy, appearing in 4 and 3 cases out of 15, respectively, indicating their potential utility in certain contexts.
%		\item For Output Type, OT\_1 and OT\_3 are almost equivalent in effectiveness, each appearing 5 and 7 times respectively out of 15. 
%		\item OT\_2 appears only once, suggesting it is less suited for pointwise ranking contexts.
%		\item It is challenging to determine the optimal choice for pointwise ranking; however, it is straightforward to identify and discard the least effective option.
%	\end{itemize}
%	
%	\item \textbf{Listwise Ranking:}
%	\begin{itemize}
%		\item TI variations are more balanced here, with TI\_1 and TI\_3 each appearing 6 times, and TI\_2 appearing 3 times out of 15. This distribution suggests no single TI dominates in effectiveness.
%		\item In terms of Output Type, TO\_2 is significantly more prevalent, appearing 12 times, indicating a strong preference or effectiveness in listwise contexts over TO\_1.
%	\end{itemize}
%	
%	\item \textbf{Setwise Ranking:}
%	\begin{itemize}
%		\item With only one TI option available, the focus shifts exclusively to Output Type. OT\_3 is noted for its superior performance, appearing in 8 out of 15 settings. This indicates its robustness and effectiveness in setwise ranking.
%		\item Conversely, OT\_2, appearing only twice, is identified as the least effective among the options.
%	\end{itemize}
%\end{itemize}
%
%These insights underscore the importance of selecting the correct ranker-specific instructions to optimize ranking algorithms across various dimensions. The distinct patterns observed suggest that while some instructions are versatile across multiple ranking types, others are uniquely suited to specific modalities, emphasizing the necessity for targeted application based on the ranking objectives and dataset characteristics.

%\subsection*{Tone Words}
%The influence of Tone Words (TW) is pervasive across various models and ranking algorithms, as evidenced in every prompt configuration analyzed. To comprehensively understand their impact, we have undertaken a detailed analysis across all settings. This investigation reveals specific trends in the utilization of TW, providing critical insights that could be instrumental in optimizing the tone settings of prompts to enhance their effectiveness. The following are the detailed observations:
%
%\begin{itemize}
%	\item \textbf{TW\_0}, which indicates the absence of any explicit tone words, appears 11 times out of 60 across all settings. This relatively low frequency suggests that while a neutral or undefined tone may suffice in contexts where the tone does not significantly impact the prompt's interpretation or user response, the inclusion of specific tone words generally enhances the effectiveness of prompts.
%	
%	\item \textbf{TW\_1}, identified as a punishing tone, occurs most frequently, being observed 15 times. This frequency implies that a direct and potentially more assertive tone can effectively align the prompt's directives with user interactions or dataset characteristics, thereby improving the performance of ranking algorithms.
%	
%	\item \textbf{TW\_2}, \textbf{TW\_4}, and \textbf{TW\_5}, which typically convey more imperative tones suggesting that rankers should only or must generate specific responses, appear with less frequency, noted 10, 9, and 7 times respectively. The forceful yet non-punitive nature of these tones in TW\_4 and TW\_5, which are succinctly expressed in just one word, may account for their lesser efficacy compared to TW\_2, which provides a more detailed directive.
%	
%	\item \textbf{TW\_3}, which denotes a polite tone, is documented 8 times. It is approximately equivalent in frequency to the less forceful tones but demonstrates lower effectiveness compared to the more direct, punishing tone.
%\end{itemize}
%
%These findings underscore the importance of incorporating tone words into prompts. The preferred choice should lean towards a punishing tone, which has demonstrated a significantly higher prevalence and effectiveness compared to other tones.
%
%
%\subsection*{Ordering}
%The organization of information, particularly the order of evidence (EO) and the position of evidence (PE), plays a crucial role in the effectiveness of ranking algorithms. Our analysis separately examines these two aspects to understand their individual and combined impacts on ranking performance. The frequencies of these configurations across different settings provide insights into their relative effectiveness:
%
%\begin{itemize}
%	\item \textbf{Evidence Order (EO)}: The configurations of \textbf{Passage First (PF)} and \textbf{Query First (QF)} appear 24 and 36 times out of a total of 60 instances, respectively. The greater prevalence of QF suggests a preference for presenting the query before the passage. This order emphasizes the query's primacy, potentially guiding the ranking algorithm to align the passage more closely with the query requirements. The higher frequency of QF indicates its effectiveness in preparing the model to better understand and respond to the query.
%	
%	\item \textbf{Position of Evidence (PE)}: Positioning evidence at the beginning of the prompt (denoted as \textbf{``B''}) appears 35 times, whereas positioning it at the end (denoted as \textbf{``E''}) appears 25 times out of 60 instances. This preference for starting with the evidence suggests that setting the initial context is crucial for guiding the interaction effectively. Beginning with the evidence draws immediate attention, helping to shape the interpretation of subsequent information and thereby enhancing the overall effectiveness of the ranking process.
%\end{itemize}
%
%These findings highlight a clear preference for presenting the query first and positioning the evidence at the beginning of the prompt. The strategic choice to emphasize the query initially and set the context early on appears to optimize the effectiveness of ranking algorithms, guiding them to better align and respond to the given prompts. This understanding can be pivotal in refining prompt configurations to achieve more accurate and relevant ranking outcomes.
%
%\subsection*{Role Playing}
%The incorporation of role-playing elements in prompts, denoted as RP, can significantly influence the effectiveness of ranking algorithms. This analysis focuses on the binary configurations of RP, where \textbf{RP\_none} indicates the absence of a role-playing sentence, and \textbf{RP\_1} signifies the inclusion of one role-playing sentence in the prompt. By examining the frequency of these configurations, we can derive insights into their relative effectiveness:
%
%\subsection*{Role Playing}
%The incorporation of role-playing elements in prompts, denoted as RP, may influence the effectiveness of ranking algorithms. This analysis focuses on the binary configurations of RP, where \textbf{RP\_none} indicates the absence of a role-playing sentence, and \textbf{RP\_1} signifies the inclusion of one role-playing sentence in the prompt. By examining the frequency of these configurations, we can derive insights into their relative effectiveness:
%
%\begin{itemize}
%	\item Out of 60 instances, \textbf{RP\_none} appears 27 times, while \textbf{RP\_1} appears 33 times. The higher frequency of RP\_1 suggests a preference for prompts that incorporate a role-playing element, indicating that adding contextual framing through role-playing can enhance performance. This implies that providing additional narrative context helps the model understand and process the prompt more effectively, whereas the absence of role-playing elements, although effective in certain contexts, is not the dominant configuration.
%\end{itemize}
%


%\section{Effectiveness of Original and Best Prompts}\label{appendix:c}
%Table~\ref{table:original-best} reports the nDCG@10 obtained by the original prompts for each ranking method and the best prompt variation for each ranking family.

% with real original prompts
%\begin{table*}[t]
%	\caption{Comparison of nDCG@10 across different rankers, LLMs and datasets. \textit{Po}: pointwise, \textit{Pa}: pairwise, \textit{Li}: listwise, \textit{Se}: setwise. \textit{Original}: the original (adapted) prompt. \textit{Best}: the best prompt found in our experiments.} 
%	\label{table:original-best}
%	\centering
%	\begin{subtable}{\textwidth}
%		\centering
%		%		\caption{Mistral-7B and Llama 3-8B}
%		\resizebox{\textwidth}{!}{
%			\begin{tabular}{llp{35pt}p{35pt}p{35pt}p{35pt}p{35pt}p{35pt}|p{35pt}p{35pt}p{35pt}p{35pt}p{35pt}p{35pt}}
%				%\toprule
%				\multirow{2}{*}{} & \multirow{2}{*}{} & \multicolumn{6}{c|}{Mistral-7B} & \multicolumn{6}{c}{Llama 3-8B} \\ \cmidrule{3-8} \cmidrule{9-14}
%				&& \multicolumn{2}{c}{DL19} & \multicolumn{2}{c}{DL20} & \multicolumn{2}{c}{COVID} & \multicolumn{2}{c}{DL19} & \multicolumn{2}{c}{DL20} & \multicolumn{2}{c}{COVID} \\ \cmidrule{3-14}
%				\multicolumn{2}{c}{Ranker}& Original & Best & Original & Best & Original & Best & Original & Best & Original & Best & Original & Best \\ \midrule
%				Po & \cite{qin2023large} & 0.5755 & \multirow{4}{*}{0.6699} & 0.4798 & \multirow{4}{*}{\textbf{0.6486}} & 0.6904 & \multirow{4}{*}{0.7988} & 0.4363 &  \multirow{4}{*}{0.5328} & 0.4517 &  \multirow{4}{*}{0.4950} & 0.7011 &  \multirow{4}{*}{0.7916}\\ %\cmidrule{3-14}
%				Po & \cite{ma2023zero} & 0.6224 &  & 0.5917 & & 0.6833 & & 0.4590 & & 0.3606 & & 0.7299 & \\ %\cmidrule{3-14}
%				Po & \cite{zhuang2023beyond}.1 & 0.6035 &  & 0.5466 & & 0.7610 & & 0.3918 & & 0.2994 & & 0.7175 & \\ %\cmidrule{3-14}
%				Po & \cite{zhuang2023beyond}.2 & 0.3699 &  & 0.3323 & & 0.5473 & & 0.4510 & & 0.3494 & & 0.7364 & \\ \midrule
%				Pa & \cite{qin2023large} & 0.5709 & 0.6450 & 0.5330 & 0.6059 & 0.7358 & 0.7738 & 0.6409 & 0.6738 & 0.5871 & 0.6340 & 0.8014 & 0.8012\\ \midrule
%				Li & \cite{ma2023zero} & 0.6602 & \multirow{2}{*}{0.6686} & 0.6043 &  \multirow{2}{*}{0.6348} & 0.7607 &  \multirow{2}{*}{0.7758} & 0.6552 &  \multirow{2}{*}{\textbf{0.7004}} & 0.6070 &  \multirow{2}{*}{\textbf{0.6619}} & 0.7156 &  \multirow{2}{*}{\textbf{0.8123}}\\ %\cmidrule{3-14}
%				Li & \cite{sun2023chatgpt} & \textit{0.6576} & & \textit{0.6105} & & 0.7605 & & \textit{0.6779} & & \textit{0.6377} & & \textit{0.8130} &\\ \midrule
%				Se & \cite{zhuang2023setwise} & 0.6517 & \textbf{0.6811} & 0.6084 & 0.6256 & \textit{0.8009} & \textbf{0.8053} & 0.6622 & 0.7000 & 0.6192 & 0.6486 & 0.7810 & 0.8035\\ \midrule
%				%				\bottomrule
%			\end{tabular}
%		}
%	\end{subtable}
%	
%	\vspace{5px}
%	
%	\begin{subtable}{\textwidth}
%		\centering
%		%		\caption{Flan-T5 Variants}
%		\resizebox{\textwidth}{!}{
%			\begin{tabular}{llp{25pt}p{25pt}p{25pt}p{25pt}p{25pt}p{25pt}p{25pt}p{25pt}p{25pt}p{25pt}p{25pt}p{25pt}p{25pt}p{25pt}p{25pt}p{25pt}p{25pt}p{25pt}}
%				
%				\multirow{2}{*}{} & \multirow{2}{*}{} & \multicolumn{6}{c}{FlanT5-Large} & \multicolumn{6}{c}{FlanT5-XL} & \multicolumn{6}{c}{FlanT5-XXL} \\ \cmidrule{3-20}
%				&& \multicolumn{2}{c}{DL19} & \multicolumn{2}{c}{DL20} & \multicolumn{2}{c}{COVID} & \multicolumn{2}{c}{DL19} & \multicolumn{2}{c}{DL20} & \multicolumn{2}{c}{COVID} & \multicolumn{2}{c}{DL19} & \multicolumn{2}{c}{DL20} & \multicolumn{2}{c}{COVID} \\ \cmidrule{3-20}
%				\multicolumn{2}{c}{Ranker}& Original & Best & Original & Best & Original & Best & Original & Best & Original & Best & Original & Best & Original & Best & Original & Best & Original & Best \\ \midrule
%				Po & \cite{qin2023large}& 0.6113 & \multirow{4}{*}{\textbf{0.6918}} & 0.5960 & \multirow{4}{*}{0.6266} & 0.6651 & \multirow{4}{*}{0.7570} & 0.6115 & \multirow{4}{*}{\textbf{0.7010}} & 0.6473 &\multirow{4}{*}{0.6727} & 0.6938 & \multirow{4}{*}{0.7742} & 0.6328 & \multirow{4}{*}{0.6860} & 0.6518 & \multirow{4}{*}{0.6733} & 0.6748 & \multirow{4}{*}{0.7784}\\ 
%				Po & \cite{ma2023zero} & 0.6410 & & 0.6062 & & 0.7001 & & 0.6733 & & 0.6512 & & 0.7348 & & 0.6615 & & 0.6516 & & 0.7326 & \\ 
%				Po & \cite{zhuang2023beyond}.1 & \textit{0.6596} & & 0.5802 & & 0.7032 & & 0.6549 & & 0.6460 & & 0.7375 &  & 0.6622 & & 0.6519 & & 0.7292 & \\ 
%				Po & \cite{zhuang2023beyond}.2 & 0.5365 & & 0.4585 & & 0.6032 & & 0.6407 & & 0.6012 & & 0.7457 & & 0.4905 & & 0.3999 & & 0.5266 & \\ \midrule
%				Pa & \cite{qin2023large} & 0.6501 & 0.6724 & \textit{0.6133} & 0.6382 & 0.7417 & 0.7788 & 0.6918 & 0.6986 & 0.6657 & 0.6823 & \textit{0.7581} & \textbf{0.7750} & 0.6807 & \textbf{0.7135} & \textit{0.6910} & \textbf{0.7126} & \textit{0.7625} & \textbf{0.7917}\\ \midrule
%				Li & \cite{ma2023zero}& 0.5058 & \multirow{2}{*}{0.6443} & 0.4802 & \multirow{2}{*}{0.6125} & 0.5960 & \multirow{2}{*}{0.7521} & 0.5730 & \multirow{2}{*}{0.6441} & 0.5675 & \multirow{2}{*}{0.6300} & 0.6377 & \multirow{2}{*}{0.7438} & 0.5785 & \multirow{2}{*}{0.7011} & 0.5621 & \multirow{2}{*}{0.6897} & 0.6482 & \multirow{2}{*}{0.7834}\\ 
%				Li & \cite{sun2023chatgpt} & 0.5522 & & 0.5292 & & 0.6532 & & 0.5921 & & 0.5706 & & 0.6630 & & 0.6843 & & 0.6656 & & 0.7381 &\\ \midrule
%				Se & \cite{zhuang2023setwise} & 0.6564 & 0.6693 & 0.6103 & \textbf{0.6525} & \textit{0.7649} & \textbf{0.7932} & \textit{0.6840} & 0.6959 & \textit{0.6762} & 0.6855 & 0.7464 & 0.7745 & \textit{0.6900} & 0.7047 & 0.6770 & 0.7036 & 0.7457 & 0.7890\\ \midrule
%				
%			\end{tabular}
%		}
%	\end{subtable}
%\end{table*}



%\begin{table*}[t]
%	\caption{Comparison of nDCG@10 across different rankers, LLMs and datasets. \textit{Po}: pointwise, \textit{Pa}: pairwise, \textit{Li}: listwise, \textit{Se}: setwise. \textit{Original}: the original (adapted) prompt. \textit{Best}: the best prompt found in our experiments. For each dataset and backbone, we highlighted in italics the best performing method that used the original prompt, and in bold the best performing method overall.} 
%	\label{table:original-best}
%	\centering
%	\begin{subtable}{\textwidth}
%		\centering
%		%		\caption{Mistral-7B and Llama 3-8B}
%		\resizebox{\textwidth}{!}{
%			\begin{tabular}{llp{35pt}p{35pt}p{35pt}p{35pt}p{35pt}p{35pt}p{35pt}p{35pt}p{35pt}p{35pt}p{35pt}p{35pt}}
%				%\toprule
%				\multirow{2}{*}{} & \multirow{2}{*}{} & \multicolumn{6}{c}{Mistral-7B} & \multicolumn{6}{c}{Llama 3-8B} \\ \cmidrule{3-8} \cmidrule{9-14}
%				&& \multicolumn{2}{c}{DL19} & \multicolumn{2}{c}{DL20} & \multicolumn{2}{c}{COVID} & \multicolumn{2}{c}{DL19} & \multicolumn{2}{c}{DL20} & \multicolumn{2}{c}{COVID} \\ \cmidrule{3-14}
%				\multicolumn{2}{c}{Ranker}& Original & Best & Original & Best & Original & Best & Original & Best & Original & Best & Original & Best \\ \midrule
%				Po & \cite{qin2023large} & 0.5851 & \multirow{4}{*}{0.6699} & 0.5237 & \multirow{4}{*}{\textbf{0.6486}} & 0.6897 & \multirow{4}{*}{0.7988} & 0.4176 &  \multirow{4}{*}{0.5328} & 0.3383 &  \multirow{4}{*}{0.4950} & 0.6678 &  \multirow{4}{*}{0.7916}\\ %\cmidrule{3-14}
%				Po & \cite{ma2023zero} & 0.6254 &  & 0.5948 & & 0.7379 & & 0.4808 & & 0.3794 & & 0.7527 & \\ %\cmidrule{3-14}
%				Po & \cite{zhuang2023beyond}.1 & 0.6414 &  & 0.5951 & & 0.7758 & & 0.3764 & & 0.3088 & & 0.7485 & \\ %\cmidrule{3-14}
%				Po & \cite{zhuang2023beyond}.2 & 0.5577 &  & 0.4896 & & 0.6967 & & 0.3890 & & 0.3466 & & 0.7242 & \\ \midrule
%				Pa & \cite{qin2023large} & 0.6263 & 0.6450 & 0.6036 & 0.6059 & 0.7724 & 0.7738 & \textit{0.6738} & 0.6738 & \textit{0.6163} & 0.6340 & \textit{0.7966} & 0.8012\\ \midrule
%				Li & \cite{ma2023zero} & 0.5863 & \multirow{2}{*}{0.6686} & 0.5492 &  \multirow{2}{*}{0.6348} & 0.7101 &  \multirow{2}{*}{0.7758} & 0.6364 &  \multirow{2}{*}{\textbf{0.7004}} & 0.6088 &  \multirow{2}{*}{\textbf{0.6619}} & 0.7393 &  \multirow{2}{*}{\textbf{0.8123}}\\ %\cmidrule{3-14}
%				Li & \cite{sun2023chatgpt} & 0.5402 & & 0.5184 & & 0.6204 & & 0.5926 & & 0.5377 & & 0.6589 &\\ \midrule
%				Se & \cite{zhuang2023setwise} & \textit{0.6567} & \textbf{0.6811} & \textit{0.6180} & 0.6256 & \textit{0.7846} & \textbf{0.8053} & 0.6733 & 0.7000 & 0.5990& 0.6486 & 0.7897 & 0.8035\\ \midrule
%				%				\bottomrule
%			\end{tabular}
%		}
%	\end{subtable}
%	
%	\vspace{5px}
%	
%	\begin{subtable}{\textwidth}
%		\centering
%		%		\caption{Flan-T5 Variants}
%		\resizebox{\textwidth}{!}{
%			\begin{tabular}{llp{25pt}p{25pt}p{25pt}p{25pt}p{25pt}p{25pt}p{25pt}p{25pt}p{25pt}p{25pt}p{25pt}p{25pt}p{25pt}p{25pt}p{25pt}p{25pt}p{25pt}p{25pt}}
%				
%				\multirow{2}{*}{} & \multirow{2}{*}{} & \multicolumn{6}{c}{FlanT5-Large} & \multicolumn{6}{c}{FlanT5-XL} & \multicolumn{6}{c}{FlanT5-XXL} \\ \cmidrule{3-20}
%				&& \multicolumn{2}{c}{DL19} & \multicolumn{2}{c}{DL20} & \multicolumn{2}{c}{COVID} & \multicolumn{2}{c}{DL19} & \multicolumn{2}{c}{DL20} & \multicolumn{2}{c}{COVID} & \multicolumn{2}{c}{DL19} & \multicolumn{2}{c}{DL20} & \multicolumn{2}{c}{COVID} \\ \cmidrule{3-20}
%				\multicolumn{2}{c}{Ranker}& Original & Best & Original & Best & Original & Best & Original & Best & Original & Best & Original & Best & Original & Best & Original & Best & Original & Best \\ \midrule
%				Po & \cite{qin2023large}& 0.6180 & \multirow{4}{*}{\textbf{0.6918}} & 0.5984 & \multirow{4}{*}{0.6266} & 0.6490 & \multirow{4}{*}{0.7570} & 0.6157 & \multirow{4}{*}{\textbf{0.7010}} & 0.6439 &\multirow{4}{*}{0.6727} & 0.6786 & \multirow{4}{*}{0.7742} & 0.6289 & \multirow{4}{*}{0.6860} & 0.6514 & \multirow{4}{*}{0.6733} & 0.6642 & \multirow{4}{*}{0.7784}\\ 
%				Po & \cite{ma2023zero} & 0.6483 & & 0.6128 & & 0.6971 & & 0.6690 & & 0.6426 & & 0.7301 & & 0.6563& & 0.6533 & & 0.7321 & \\ 
%				Po & \cite{zhuang2023beyond}.1 & 0.6468 & & 0.5698 & & 0.6672 & & 0.6300& & 0.6444 & & 0.7023 &  & 0.6451 & & 0.6274 & & 0.6983 & \\ 
%				Po & \cite{zhuang2023beyond}.2 & 0.5164 & & 0.4387 & & 0.6206 & & 0.6054 & & 0.5971 & &0.7095 & & 0.4068 & & 0.3301 & & 0.4335 & \\ \midrule
%				Pa & \cite{qin2023large} & \textit{0.6677} & 0.6724 & \textit{0.6237} & 0.6382 & \textit{0.7558} & 0.7788 & \textit{0.6845} & 0.6986 & \textit{0.6766} & 0.6823 & 0.7536 & \textbf{0.7750} & 0.6915 & \textbf{0.7135} & \textit{0.6992} & \textbf{0.7126} & 0.7452& \textbf{0.7917}\\ \midrule
%				Li & \cite{ma2023zero}& 0.5465 & \multirow{2}{*}{0.6443} & 0.5081 & \multirow{2}{*}{0.6125} & 0.6067 & \multirow{2}{*}{0.7521} & 0.5688 & \multirow{2}{*}{0.6441} & 0.5576 & \multirow{2}{*}{0.6300} & 0.6312 & \multirow{2}{*}{0.7438} & 0.5915 & \multirow{2}{*}{0.7011} & 0.5852 & \multirow{2}{*}{0.6897} & 0.6955 & \multirow{2}{*}{0.7834}\\ 
%				Li & \cite{sun2023chatgpt} & 0.6199 & & 0.5552 & & 0.7445 & & 0.6129 & & 0.5966 & & 0.6938 & & 0.6920 & & 0.6672 & & \textit{0.7736} &\\ \midrule
%				Se & \cite{zhuang2023setwise} & 0.6503 & 0.6693 & 0.5754 & \textbf{0.6525} & 0.7440 & \textbf{0.7932} & 0.6812 & 0.6959 & 0.6747 & 0.6855 & \textit{0.7540} & 0.7745 & \textit{0.6925} & 0.7047 & 0.6776 & 0.7036 & 0.7617 & 0.7890\\ \midrule
%				
%			\end{tabular}
%		}
%	\end{subtable}
%\end{table*}
